# Supplementary material for: Homotopic Action: A Pathway to Convergent Diagrammatic Theories
Source: arXiv:2010.05301 ancillary file (2021-06-23)
Supplement: Supplementary file 1 [file supplemental_material.pdf]

# Supplemental Information
# Homotopic Action: A Pathway to Convergent Diagrammatic Theories

Aaram J. Kim,[1] Nikolay V. Prokof'ev,[2] Boris V. Svistunov,[2,3,4] and Evgeny Kozik[1]

[1] *Department of Physics, Kings College London, Strand, London WC2R 2LS, UK*
[2] *Department of Physics, University of Massachusetts, Amherst, MA 01003, USA*
[3] *National Research Center Kurchatov Institute," 123182 Moscow, Russia*
[4] *Wilczek Quantum Center, School of Physics and Astronomy and T. D. Lee Institute, Shanghai Jiao Tong University, Shanghai 200240, China*

## I. Computation time

DiagMC typically computes directly the series coefficients $a_n$ (for the original action) or $b_n$ (for the homotopic action). We thus need to determine the optimal number of (effective, i.e. including the autocorrelation time) Monte Carlo (MC) steps $N^*_{\rm MC}(n)$ needed for computing the coefficient at each diagram order $n$ in order to obtain the partial sum $\sum_{n=0}^N a_n$ or $\sum_{n=0}^N b_n w_*^n$ with the smallest statistical error $\delta\varepsilon$ for a given fixed simulation time $T_{\rm cpu}$. To this end, we introduce the formal function $\delta\varepsilon(N;\lambda)$ with the Lagrange multiplier $\lambda$,

$$\delta\varepsilon^2(N;\lambda) = \sum_{n=0}^{N} \frac{\gamma(n)}{N_{\rm MC}(n)} + \lambda\left(\sum_{n=0}^{N}\tau(n)N_{\rm MC}(n) - T_{\rm cpu}\right) . \qquad (1)$$

The term under the first sum is the statistical variance of the MC sampling of the order-$n$ coefficient, which is inversely proportional to the arbitrary at this point number of effective MC steps $N_{\rm MC}(n)$ with the prefactor $\gamma(n)$, and $\tau(n)$ is the time that each (effective) MC step takes at order $n$. At the minimum of $\delta\varepsilon^2(N;\lambda)$ is reached at the following distribution of the MC steps

$$N^*_{\rm MC}(n) = \frac{T_{\rm cpu}}{\sum_{j=0}^N \sqrt{\tau(j)\gamma(j)}}\sqrt{\frac{\gamma(n)}{\tau(n)}} \qquad (2)$$

and its value is

$$\delta\varepsilon_*^2(N) = \frac{\left(\sum_{n=0}^N \sqrt{\tau(n)\gamma(n)}\right)^2}{T_{\rm cpu}} . \qquad (3)$$

In addition to the statistical error of the partial sum, there is a *systematic* error $\delta\varepsilon_{\rm sys}(N)$ due to the truncation of the series at order $N$. We define the total computation time $T^*_{\rm cpu}(N)$ as the minimal time required to reach the stochastic error $\delta\varepsilon_*(N)$ that is equal to the systematic error $\delta\varepsilon_{\rm sys}(N)$, which thus reads

$$T^*_{\rm cpu}(N) = \frac{\left(\sum_{n=0}^N \sqrt{\tau(n)\gamma(n)}\right)^2}{\delta\varepsilon_{\rm sys}(N)^2} . \qquad (4)$$

The prefactor $\gamma(n)$ is the only scheme-dependent parameter (apart from an insignificant difference in $\tau(n)$, see below), which is responsible to the efficiency gain when using the homotopic action. The formal power series of the physical quantity $A$ (in our case the number density) is written as

$$A \widehat{=} \begin{cases} \sum_n a_n\xi^n = \sum_{nm} a_m M_{mn} w^n \ , & \text{(original action)} \\ \sum_n b_n w^n \ , & \text{(homotopic action)} \end{cases} \qquad (5)$$

where $M_{mn}$ defines the conformal transformation, $b_n = \sum_m a_m M_{mn}$ . The corresponding statistical variance of the power series has the following form

$$\delta A^2 = \begin{cases} \sum_{nm} \delta a_m^2 M_{mn}^2 w^{2n} \ , & \text{(original action)} \\ \sum_n \delta b_n^2 w^{2n} \ . & \text{(homotopic action)} \end{cases} \qquad (6)$$

The MC variance of $a_n$ and $b_n$ can be expressed as $z_n^2(1-\langle{\rm sign}\rangle_n^2)/N_{\rm MC}(n)$ where $z_n$ is the absolute-value integral of the corresponding MC configuration weight over the configuration space and $\langle{\rm sign}\rangle_n$ is the average sign[1]. By identifying $\delta A^2$ with the first term of Eq. (1), one can extract the expression for $\gamma(n)$ as follows:

$$\gamma(n) \simeq \begin{cases} \sum_m z_{a,m}^2(1-\langle{\rm sign}_a\rangle_n^2)M_{mn}^2 w^{2n} \ , & \text{(original action)} \\ z_{b,n}^2(1-\langle{\rm sign}_b\rangle_n^2)w^{2n} \ . & \text{(homotopic action)} \end{cases} \qquad (7)$$

We directly measure $z_n$, $\langle{\rm sign}\rangle_n$, and $\tau(n)$ for both schemes during the MC sampling. Figure S1 shows the actual dependence $\tau(n)$ in our implementation of both

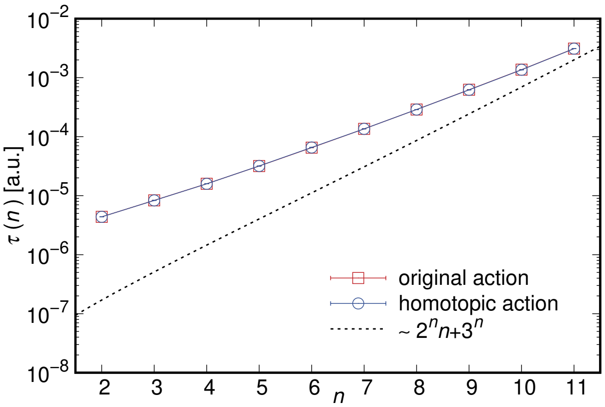


Figure S1: Scaling with the diagram order $n$ of the time that one MC step takes in our implementation of the two schemes for the density series in the $2d$ Hubbard model at $T = 0.2t$, $U = 7t$, $\mu = 1.8959t$ (the parameter set of Fig. 3 of the main text).

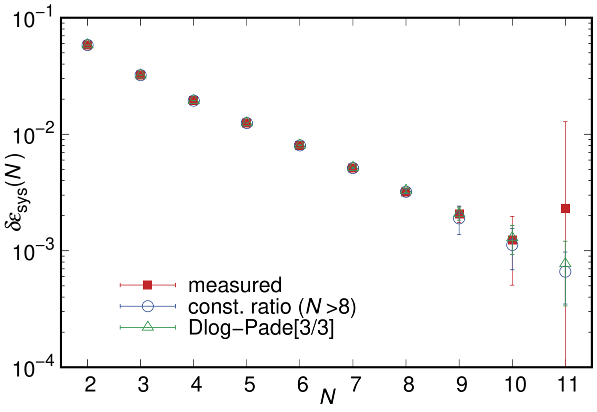


Figure S2: The systematic error $\delta\varepsilon_{\rm sys}$ as a function of the truncation diagram order $N$ for the parameters of Fig. S1. We compare the measured $\delta\varepsilon_{\rm sys}$ with two different extrapolation schemes – an extrapolation assuming that $b_{n-1}/b_n$ becomes independent of $n$ for $n > 8$ (blue circles) and the Dlog-Padé approximant of order $[3/3]^3$ (green triangles).

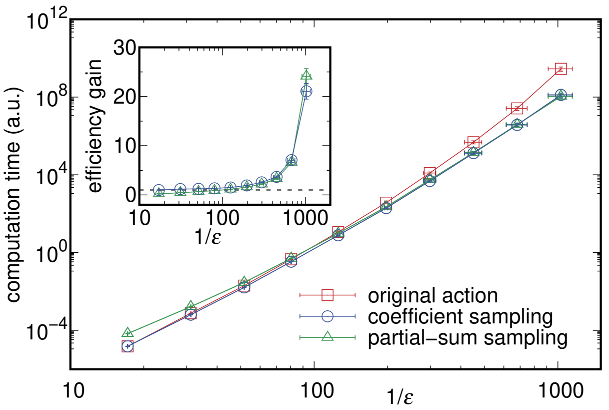


Figure S3: Computation time (in arbitrary unit) required to achieve the systematic error $\varepsilon$ for three different methods: the convergent series generated by the original action post-processed by the conformal mapping, the coefficient sampling and the partial-sum sampling within the homotopic action. The inset presents the efficiency gain of two different implementations of the homotopic action compared to the original action as a function $1/\varepsilon$. The same parameter set as in Fig. 3 of the main text is used.

schemes. It follows an approximately exponential scaling approaching the (moderate-$n$) theoretical estimate[2] $O(n2^n) + O(3^n)$. Importantly, we can observe that the difference in the time per one MC step between the CDet schemes based on the original and homotopic action is negligible.

Finally, the systematic error $\delta\varepsilon_{\rm sys}$ is estimated as the difference between the result obtained by an extrapolation of $\sum_n b_n w_*^n$ to infinite order using the Dlog-Padé method[3] and the one of the truncated partial sum. Figure S2 shows the exponential decrease of $\delta\varepsilon_{\rm sys}(N)$.

## II. Direct sampling of the partial sum

One of fascinating features of the homotopic action combined with the CDet algorithm is that the partial sum of the series can be directly sampled without additional computational cost. For a fixed set of $N$ internal vertices, over the positions of which the MC integration is performed, the sum of all diagrams contributing to $\sum_{n=0}^N b_n w_*^n$ plays a role of the stochastic weight for MC updates. In our implementation, when evaluating the diagrams at $n < N$ we average them over all possible subsets of $n$ vertices out of the given $N$ ones.

The total computational time for this scheme is given, following Sec. I, by

$$T^*_{\rm cpu}(N) = \frac{\tau(N)\gamma(N)}{\delta\varepsilon_{\rm sys}(N)^2} \ , \qquad (8)$$

where $\gamma(N) = z^2_{p,N}(1 - \langle {\rm sign}\rangle^2_N)$ . In Fig. S3, the computation time is compared for the three different methods: the CDet calculation of the coefficients $a_n$ (original action) with the subsequent resummation of the divergent series by the conformal map $w(\xi)$, calculation of the $b_n$ coefficients of the convergent series using the homotopic action formalism (coefficient sampling), and direct sampling of the contributions to $\sum_{n=0}^N b_n w_*^n$ (partial-sum sampling). While the partial-sum sampling is the least efficient in low orders, it is the most efficient starting from the diagram order 11. Reduction of the computational time by the partial-sum-sampling scheme compared to the original-action and coefficient-sampling schemes happens at orders 6 and 11 respectively, suggesting that partial-sum sampling is the most promising scheme for high-order calculations. The fact that there is no need to manually distribute the CPU time between the diagram orders optimally is a another practical benefit of sampling the partial sum directly.

## III. Covariance analysis

The scheme based on the homotopic action enables a cancellation of the sign-alternating diagrammatic contributions of different orders, which nearly compensate in the final answer, at the level of the MC sampling. The extent of this cancellation can be detected and quantified by the correlation function between the diagrammatic contributions of different orders. To this end, we define the covariance matrix

$${\rm Cov}^{(k)}(i,j) = M_{ik}M_{jk}\left(\langle a_i a_j\rangle - \langle a_i\rangle\langle a_j\rangle\right) \ , \qquad (9)$$

which measures the correlation between all the original-action diagrams of orders $i$ and $j$ as they contribute to the MC sampling for the coefficient $b_k$. Here, $\langle \dots \rangle$ stands

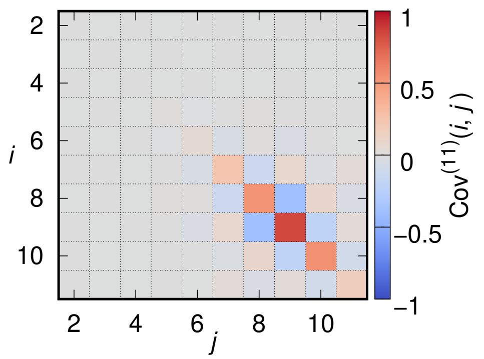


Figure S4: Color map of the normalized covariance matrix while calculating the density series of order 11. We choose the same parameters as in Fig. 3 of the main text. The definition of the covariance matrix $\mathrm{Cov}^{(k)}(i,j)$ is written in Eq. (9). We normalize $\mathrm{Cov}^{(k)}(i,j)$ by $\delta b_k^2$ . The covariance of the diagonal elements is peaked in the intermediate diagram order, in this case 9th order. And the sub-diagonal elements give negative contribution to the total error which leads to the error gain of the homotopic action.

for the Monte Carlo average during the calculation based on the homotopic action.

Figure S4 shows the covariance matrix $\mathrm{Cov}^{(11)}(i,j)$ for $k = 11$ demonstrating the clear negative correlations, particularly between the neighboring orders $i$ and $j$. The off-diagonal elements show the checkerboard-like sign pattern, but the negative sub-diagonal elements around order 9 are prominent. The degree of correlation decays away from the diagonal, so that the total contribution from the off-diagonal elements is negative.

Since the MC variance of $b_k$ for sampling with the homotopic action is written as

$$\delta b_k^2 = \sum_{i,j} \mathrm{Cov}^{(k)}(i,j) \ , \tag{10}$$

the net negative contribution from the off-diagonal elements leads to the error reduction. In contrast, when the convergent series is obtained by post-processing in the scheme based on the original action, $a_n$ coefficients of different orders are sampled independently, so that the variance of the resulting $b_k$ coefficient becomes $\sum_j \mathrm{Cov}^{(k)}(j,j)$ without the contribution of the negative correlations from the off-diagonal elements.

## IV. Anti-collapse regularization of the interaction

Here we work in the momentum space, and our idea is to continuously deform the original interaction term, which is a sum over momenta $\{\mathbf{p}\}$ of all fields involved, $S_{\mathrm{int}} = \sum_{\{\mathbf{p}\}} \mathcal{S}_{\mathrm{int}}(\{\mathbf{p}\})$, suppressing contributions from large momenta. Let $p_*$ be the magnitude of the largest momentum in a given set $\{\mathbf{p}\}$. Define an integer-valued function

$$f(p_*) = 1, \quad \text{if} \quad p_*/p_0 \le \nu,$$
$$f(p_*) = j, \quad \text{if} \quad \nu^{j-1} < p_*/p_0 \le \nu^j \quad (j = 2,3,4,\ldots),$$

where $p_0$ is the momentum unit, and $\nu > 1$ is a dimensionless real number. The transformation

$$S_{\mathrm{int}} \to \bar{S}_{\mathrm{int}}(w) = \sum_{n=0}^{\infty} (w/w^*)^n \sum_{\{\mathbf{p}\}} \delta_{n,f(p_*)} \, \mathcal{S}_{\mathrm{int}}(\{\mathbf{p}\}) \, , \tag{11}$$

exponentially suppresses coupling to large momenta at $|w/w_*| < 1$, but recovers the original interaction at $w = w_*$. It is key that the largest contribution to the action density from $\mathcal{S}_{\mathrm{int}}(\{\mathbf{p}\})$ cannot exceed $\propto (p_*/p_0)^\alpha$ in the UV limit due to the Pauli exclusion principle, $\alpha$ being a fixed positive exponent. Therefore, regularization (11) limits the contribution (per unit volume) of the $n$-th order of the expansion of $\bar{S}_{\mathrm{int}}(w)$ in the powers of $w$ to $\propto (w/w_*)^n \nu^{\alpha n}$, eliminating the collapse for $|w| < \nu^{-\alpha}$. Similarly, for bosonic/classical fields, one can employ the regularization protocol of Ref.[4] to construct a sequence of actions $S_N$ with the interaction terms designed to vanish in the large field-amplitude limit and converging to the physical action for $N \to \infty$.


[1] R. Rossi, N. Prokof'ev, B. Svistunov, K. Van Houcke, and F. Werner, EPL **118**, 10004 (2017).
[2] F. Šimkovic and E. Kozik, Phys. Rev. B **100**, 121102 (2019).
[3] G. A. Baker Jr, Phys. Rev. **124**, 768 (1961).
[4] L. Pollet, N. V. Prokof'ev, and B. V. Svistunov, Phys. Rev. Lett. **105**, 210601 (2010).
